# Supplementary material for: Directionality measures in evolutionary ecological networks: Insights from the Tangled Nature model
Source: arXiv:2507.14062 source file (2025-07-18)
Supplement: Supplementary file 1 [file S1_Appendix.pdf]

# Directionality measures in evolutionary ecological networks: Insights from the Tangled Nature model

Andrea Marchetti, Henrik Jeldtoft Jensen

# Supporting Information S1 Appendix

## Mathematical details

### Network entropy and number of paths

Consider an undirected, unweighted graph whose adjacency matrix is given by $A$. Let $\Omega^{(t)}$ be the set of possible paths $(x_0, \ldots, x_t)$ of length $t+1$ on the network, and let $\mu_t$ be a probability measure on $\Omega^{(t)}$. When $t$ is large, the paths in $\Omega^{(t)}$ will fall into two classes, depending on their frequency [1]: a class $S_1$ in which all paths have approximately the same frequency, and a class $S_2$ whose paths have probabilities that sum to $\epsilon$.

We define by $N^*(t)$ the minimal number of paths generated up to time $t$ whose measure exceeds $1-\epsilon$; this corresponds to the typical number of distinct paths that can be explored up to time $t$ [1]. Then, we denote by $W^* = \lim_{t\to\infty} [N^*(t)]^{1/t}$ the typical number of distinct infinite paths. It can be shown [1, 2] that $H = \log W^*$, that is, network entropy counts the number of distinct infinite paths in the network.

### The Fluctuation-Stability Theorem

Consider a networked dynamical system subject to perturbations arising from changes in its dynamical rules or its topology [3]. Let $P_\epsilon(t)$ denote the probability that, at time $t$, the mean of a given observable deviates more than $\epsilon$ from its unperturbed value. We define the fluctuation decay rate $R$ as the asymptotic convergence of $P_\epsilon(t)$ to 0 on a logarithmic scale [3, 4]:

$$R \equiv \lim_{t\to\infty} \left[ -\frac{1}{t} \log P_\epsilon(t) \right]. \tag{1}$$

In this sense, $R$ characterises the insensitivity of an observable to structural or dynamic changes in the underlying parameters [3].

Consider now a small perturbation $\delta$, so that the network's adjacency matrix transforms as $\mathbf{A}(\delta) = (A_{ij})^{1+\delta}$. We denote by $H(\delta)$ and $R(\delta)$ the entropy and fluctuation decay rate of the perturbed network, respectively. We also define $\Delta H = H(\delta) - H(0)$, $\Delta R = R(\delta) - R(0)$. The following theorem holds [3, 4].

> **Theorem (Fluctuation-Stability).** For a sufficiently small perturbation $\delta$, variations in network entropy and fluctuation decay rate are positively correlated:
>
> $$\Delta H \Delta R > 0. \tag{2}$$

The theorem can be interpreted as follows: any changes that promote stabilisation of the network around its stationary configuration will lead to a decrease in entropy, whereas changes that slow the convergence of an observable to its stationary state – potentially causing it to escape its basin of attraction and settle into a different steady-state solution – will result in an increase in entropy.

## Calculation of the clustering coefficient

To calculate the global clustering coefficient, we have employed the dedicated Python's built-in function from the package NetworkX. This computes the local clustering coefficient $c_i$ for all nodes and then calculates the average $C$, returning

$$C = \frac{1}{n} \sum_i c_i, \tag{3}$$

where $n$ is the number of nodes in the graph. In particular, the formula for the local clustering coefficient in a directed binary network [5] is

$$c_i = \frac{\left[(A + A^T)^3\right]_{ii}}{2\left[d_i^{tot}\left(d_i^{tot} - 1\right) - 2d_i^{\leftrightarrow}\right]} \tag{4}$$

where $A$ is the adjacency matrix, $d_i^{tot}$ is the total degree of $i$, and $d_i^{\leftrightarrow}$ is the reciprocal degree of $i$. The total degree is defined as the total number of incoming or outgoing edges $d_i^{tot} = \sum_{j \neq i} A_{ij} + \sum_{j \neq i} A_{ji}$, while the reciprocal degree is defined as the number of bilateral edges $d_i^{\leftrightarrow} = \sum_{j \neq i} A_{ij} A_{ji} = \left(A^2\right)_{ii}$.

# References


1. Demetrius LA. Boltzmann, Darwin and Directionality theory. Physics Reports. 2013;530:1–85. doi:10.1016/j.physrep.2013.04.001.

2. Demetrius L, Gundlach V. Directionality Theory and the Entropic Principle of Natural Selection. Entropy. 2014;16:5428–5522. doi:10.3390/e16105428.

3. Demetrius L, Manke T. Robustness and network evolution—an entropic principle. Physica A: Statistical Mechanics and its Applications. 2005;346:682–696. doi:10.1016/j.physa.2004.07.011.

4. Demetrius L, Gundlach VM, Ochs G. Complexity and demographic stability in population models. Theoretical Population Biology. 2004;65:211–225. doi:10.1016/j.tpb.2003.12.002.

5. Fagiolo G. Clustering in complex directed networks. Physical Review E. 2007;76:026107. doi:10.1103/PhysRevE.76.026107.
